# Supplementary material for: Stable Object Reorientation using Contact Plane Registration
Source: arXiv:2208.08962 source file (2022-08-18)
Supplement: Supplementary file 1 [file appendix.tex]

\section*{APPENDIX}
\subsection{Calculating the rotation matrix that rotates vector $\myvec{s}$ onto vector $\myvec{t}$ \cite{moller1999efficiently}}
% We provide a simple exposition of the formula for calculating the relative rotation from vector $\myvec{s}$ to vector $\myvec{t}$ .
\label{Rodrigues'_rot_2_vecs}
\begin{enumerate}
    \item Calculate the axis of rotation $\myvec{u}$ by taking the cross product between $\myvec{s}$ and $\myvec{t}$: $\myvec{u} = \myvec{s} \times \myvec{t}$
    \item Find the planar rotation that rotates $\myvec{s}$ about $\myvec{u}$ until $\myvec{s}$ aligns with $\myvec{t}$. The smallest such rotation angle is $\theta = \arccos{(\myvec{s} \cdot \myvec{t})}$ and is related to $\myvec{s}$ and $\myvec{t}$ by the following equations: $\sin(\theta) = |\myvec{s} \times \myvec{t}|$, $\cos(\theta) = \myvec{s} \cdot \myvec{t}$
    \item The Rodrigues' formula for converting from an axis-angle rotation to a rotation matrix is as follows: $R(\theta, \myvec{u}) = I + [\myvec{u}]_\times + \frac{1 - \cos(\theta)}{\sin^2(\theta)} [\myvec{u}]_\times^2$ where $[\bullet]_\times$ is the skew-symmetric cross-product operator.
    % that allows rewriting the cross product $\myvec{u} \times \myvec{s}$ as a matrix-vector multiplication $[\myvec{u}]_\times \myvec{s}$. \\
    % We plug in $\myvec{s}$ and $\myvec{t}$ into the Rodrigues' formula to get the rotation matrix $R$ that rotates $\myvec{s}$ to $\myvec{t}$.
    We plug in the right-hand-side terms for $\myvec{u}$, $\cos{\theta}$, $\sin{\theta}$ into the Rodrigues' formula to get the rotation matrix $R$ as a function of $\myvec{s}$ and $\myvec{t}$.
    \item We rewrite the above formula as: $R(\theta, \myvec{u}) = I + [\myvec{u}]_\times + \frac{1}{1 + \cos{\theta}} [\myvec{u}]_\times^2$ using the following equality: $\frac{1 - \cos{\theta}}{\sin^2(\theta)} = \frac{1 - \cos{\theta}}{1- \cos^2{\theta}} = \frac{1}{1 + \cos{\theta}}$.
    The rewritten formula clearly fails when $\cos{\theta} = -1$ i.e. when $\myvec{s}$ and $\myvec{t}$ are antiparallel. To resolve this failure case, when $\myvec{s}$ and $\myvec{t}$ are antiparallel we set $R$ equal to a $180^{\degree}$ rotation about the world frame x-axis (recall that the object is centered at the world frame origin). 
    % as a function of $\myvec{s}$ and $\myvec{t}$. 
\end{enumerate}

\subsection{Full stacking policy + rotation function}
\label{stacking_policy}
We utilize a hand-scripted policy to designate both the order of objects to be stacked as well as the translations to apply to the objects. Then, the various methods for producing relative rotation from pointcloud in Section \ref{sec:results} are implemented in function $f$ to rotate each object to a stable and height-maximizing orientation (Algorithm \ref{alg: stacking_policy}). While we are working in simulation and can assume ground truth knowledge of the centers of mass, pointcloud object segmentation, and object type labels, existing methods can be used to regress and classify these quantities \cite{qi2019deep}. 

\begin{figure}[!t]
 \removelatexerror

\begin{algorithm}[H]
\caption{Stacking policy}
\label{alg: stacking_policy}
  \begin{algorithmic}[1]
\State \textbf{Input:} Segmented pointclouds $\{ X_i \}$, Object IDs $\{ i \}$, Centers of mass $\{p_i \}$, Object type labels $\{ A_i \}$, Max timesteps $T$, Visited object IDs array $V$, Rotation function $f$ \hspace{20mm}
\vspace{10pt}

\For{timestep $t$ in 1, ... , $T$}
    \State support\_block\_id = SampleSupportBlock($\{ A_i \}$, $\{ i \}$)
    \If{support\_block\_id is not None}:
        \State next\_block\_id = support\_block\_id
    \Else
        \State next\_block\_id = GetCapstoneBlock($\{ A_i \}$, $\{ i \}$)
    \EndIf
    \State centered\_pointcloud = $X_{\text{next\_block\_id}}$ - $p_{\text{next\_block\_id}}$
    \State $R$ = $f$(centered\_pointcloud)
    \State ApplyRotation(next\_block\_id, $R$)
    \State TranslateOntopExistingTower(next\_block\_id, $V$)
    \State StepEnvironmentAndUpdateVariables()
\EndFor
\end{algorithmic}
\end{algorithm}

\end{figure}

% There are two object types: ``support" and ``capstone". A support block is a block with two flat faces with antiparallel normals, where each face is wide enough to support an additional block on top. A capstone block is a block without this property, and thus does not support further stacking. Capstone blocks are placed as the last block, at the very top of the tower. Support and capstone blocks are labelled by hand, and these labels are provided to the policy. We assume there is at most one capstone block in the environment for any given episode.

The function for translating the stacking object is $\tt{TranslateOntopExistingTower}$. This subroutine moves the stacking object, from a position above the tower, downwards until contact is detected with the tower, then releases the object. For real world manipulation, this procedure would roughly correspond with using a force-torque sensor at the end-effector to detect contact between the gripped object and the existing tower, before releasing the object from the gripper. The $XY$-coordinates of the initial position are set to $XY$-coordinates of the aggregate center of mass of all the existing objects in the tower.  After the object is released, the simulator is stepped forward.
